# Supplementary material for: jBOT: Semantic Jet Representation Clustering Emerges from Self-Distillation
Source: arXiv:2601.11719 source file (2026-09-18)
Supplement: Supplementary file 1 [file sec_appendix.tex]

\section{Appendix}
\label{sec:appendix}
